# Supplementary material for: Gemini: Integrating Full-fledged Sensing upon Millimeter Wave Communications
Source: arXiv:2407.04174 source file (2024-10-22)
Supplement: Supplementary file 1 [file appendix.tex]

\noindent{\Large \bf Appendix}

\vspace{-1ex}
\section{Beamforming Training in IEEE 802.11ay} \label{append:a}
\vspace{-0.5ex}
\rev{In this section, we introduce the beamforming training procedure in IEEE 802.11ay~\cite{802_11ay} as the additional description for the sector sweep phase in Section~\ref{ssec:background}.
To find the best beam alignment between AP and UE, there are the AP-side and UE-side sweep stages as illustrated in Figure~\ref{fig:beamtraining}. At the AP-side sweep stage, the AP transmits SSW frames with Tx sector IDs sequentially to the UE with quasi-omni-directional pattern, and it responses the best Tx sector ID to the AP. Secondly, the operations of the the AP-side sweep stage are reversed at the UE-side sweep stage. Hereby, both beams of the AP and UE are aligned.  

% To find the best-beamformed link, AP should complete two phases: Sector-level sweep (SLS) phase, and Beam Refinement Protocol (BRP) phase, as illustrated in Figure~\ref{fig:beamtraining}.

% \textbf{ 1) Sector-level Sweep:} Initially, the AP transmits SSW frames to train its TX sectors. The UEs respond by transmitting their SSW frames to the AP, embedding the best sector ID. Afterward, the AP directs the beam toward the optimal TX sector's direction.

%
% \textbf{ 2) Beam Refinement Protocol:} Following the SLS, AP found the best beam direction, and the BRP phase trains the RX sectors. AP transmits BRP frames in a quasi-omni direction, and the UE receives the frames through different sectors to determine the best RX sector.

% After two phases, AP and UE complete the beam alignment and find the best communication link.
}

\begin{figure}[h]
%\vspace{-1ex}
  \setlength\abovecaptionskip{8pt}
  \centering
  \includegraphics[width=1\columnwidth]{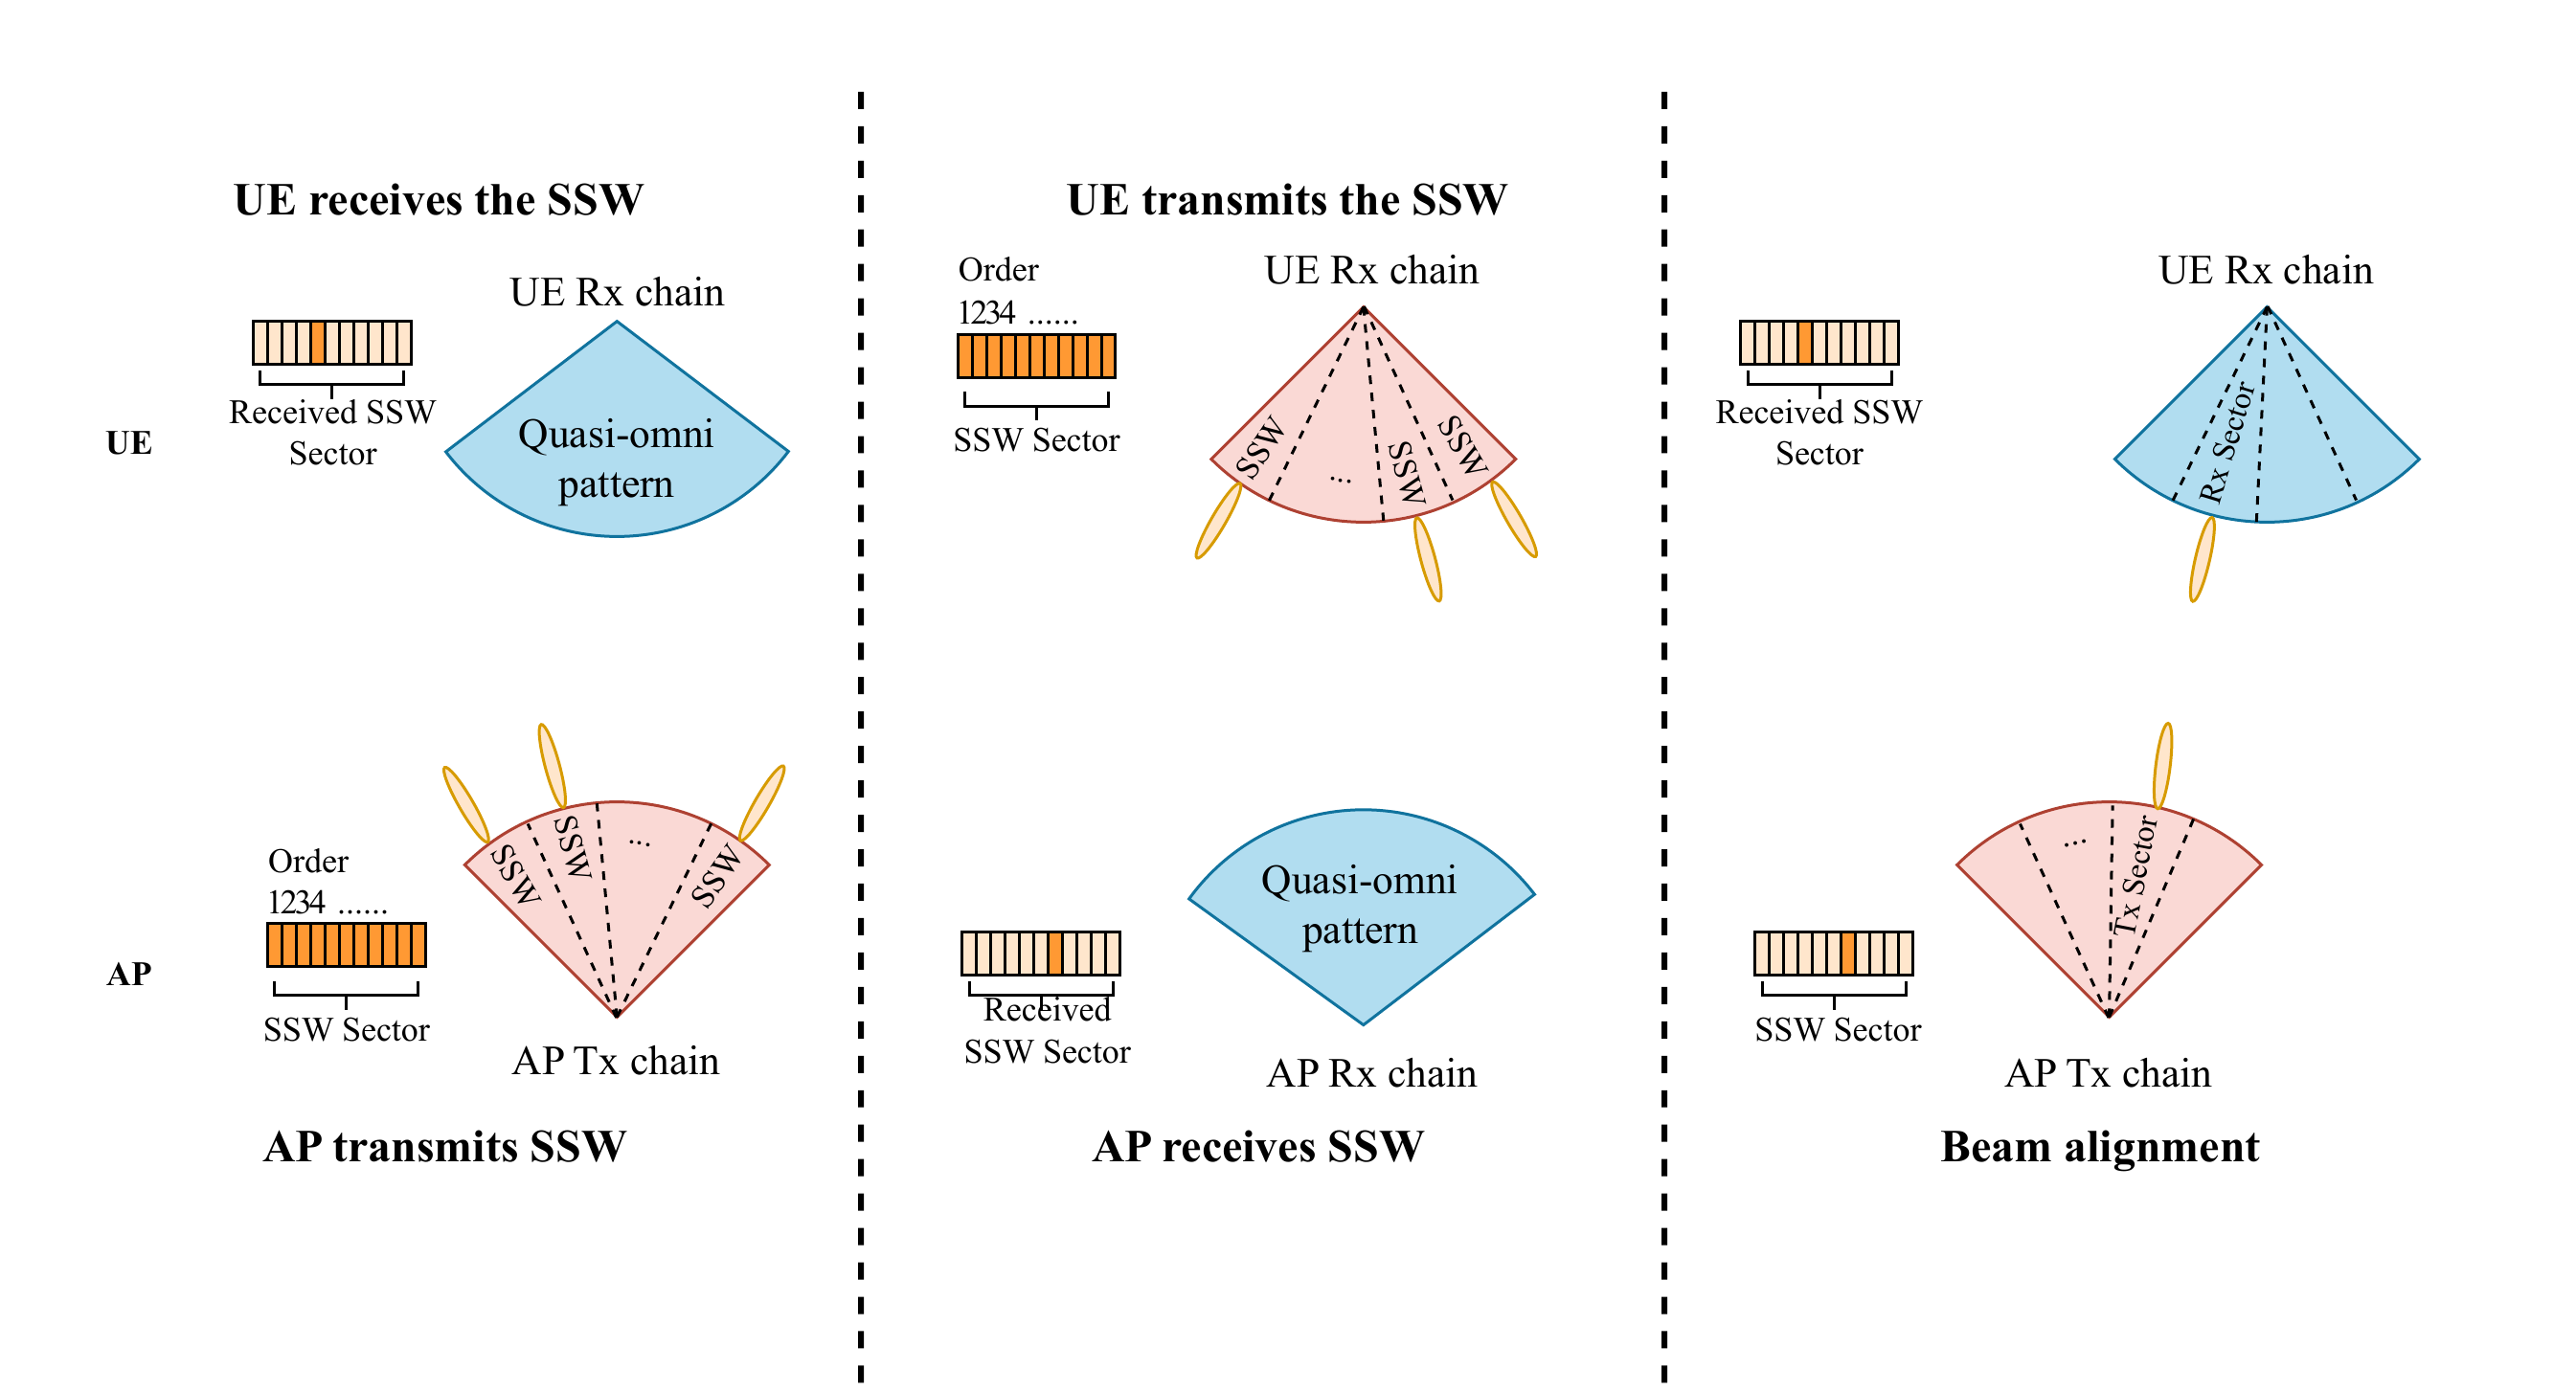}
  % \vspace{-0.3cm}
  \caption{Brief procedure of beamforming training.}
  \label{fig:beamtraining}
%  \vspace{-1ex}
\end{figure}

\vspace{-1ex}
\section{Implementation Details} \label{append:b}
\vspace{-0.5ex}
%For implementation details
\rev{
Supplemental implementation details for \name are described in the following.
\vspace{-1ex}
\paragraph{MmWave Frontend:}\name's mmWave frontend employs BF\/01~\cite{SiversBF01_2021} that is 16-antenna phased array. That phased array's amplitude and phase of each antenna can be controlled via AWV look-up table via serial peripheral interface bus in real time.

% The 60GHz mmWave frontend TRX BF\/01~\cite{SiversBF01_2021} equips 16 Rx and 16 Tx antennas. In Tx and Rx modes,  the module controls the amplitude and phase of 16 antennas through the Antenna Weight Vector Look-up Table (AWV LUT), configurable with up to 64 beam patterns via SPI, including the quasi-omnidirectional pattern. Users can directly program their self-defined beam patterns into the frontend for real-time beam alignment.

%
%

% \textbf{CIR estimation:} Our packet structure adheres to IEEE 802.11ay~\cite{802_11ay}, retaining its native packet structure. Beam training (TRN) fields are appended to packets to enable CIR estimation during communication. 
%
\vspace{-1ex}
\paragraph{Baseband Processing Unit:}\name adopts Zynq UltraScale+ RFSoC ZU48DR board~\cite{xilinxzcu208} as \name's baseband processing unit. The RFSoC board integrates 14-bit 5~\!GSPS ADCs and 14-bit 10~\!GSPS DACs for wideband signal processing. It also has a processing system with quad-core Cortex-A53, real-time Cortex-R5 processors, and 930k logic cell. \name builds on the opensource MIMORPH project~\cite{MIMORPH-MobiSys21}, but implements additional components based on Section~\ref{sec:design}. 

% \paragraph{Firmware:} 
% The firmware leverages components from the open-source MIMORPH project~\cite{MIMORPH-MobiSys21} and is implemented on Xilinx RFSoC boards~\cite{xilinxzcu208}. 
%
% The Xilinx RFSoC utilizes an UltraScale+ ZU48DR, integrating 14-bit 5GSPS ADCs and 14-bit 10GSPS DACs for wideband signal processing. The RFSoC incorporates a Processing System (PS) with quad-core Cortex-A53, real-time Cortex-R5 processors, along with 930k logic cell UltraScale+ programmable logic (PL).

%It also includes a PS with a quad-core ARM Cortex-A53 processor and an ARM R5 real-time processor, and the UltraScale+ programmable logic (PL) subsystem comprises 930k FPGA logic cells.
%
% The Xilinx RFSoC hardware resources were fully utilized. One Cortex-A53 core handled system control. The remaining Cortex-A53 and Cortex-R5 cores were allocated for tasks including protocol functionality, beamforming, and calibration as elaborated in Section~\ref{sec:design}. 
%
\vspace{-1ex}
\paragraph{PC Host:}We deploy a lightweight TCP/IP stack (lwIP)~\cite{lwIPL_2011} in RFSoC board, enabling communication with a host PC through Ethernet. We also implement UDP interface in MATLAB to configure and communicate with the RFSoC board for research convenience. In the meanwhile, the deep neural network for interference cancellation is trained on an Nvidia RTX 3080Ti.
%
% With this, we can configure the platform and develop functions in MATLAB for research convenience.
%
% Both sensing and beam scheduling are implemented within Matlab. In the meanwhile, the deep neural network for interference cancellation is trained on an Nvidia RTX 3080Ti.
}

\vspace{-1ex}
\section{Simulations for Large-scale Deployment} \label{append:c}
\vspace{-1ex}
% Our experimental setup is based on 1 AP, 1UE for a single subject~\ref{sec:eval}.  
% Given the experimental platform's high cost, we cannot evaluate \name in a full-scale deployment. 
%
% \begin{figure}[h]
% \vspace{-.5ex}
% \setlength\abovecaptionskip{3pt}
% \centering
% \subfigure[\rev{One AP with different UEs.}]{
%     \includegraphics[width=0.228\textwidth]{figures/simulation/simulation1APThroughput.pdf}
%     \label{fig:sim1AP}
% }
% % \hspace{.1cm}
% \subfigure[\rev{50 UEs with different APs.}]{
%     \includegraphics[width=0.223\textwidth]{figures/simulation/simulationAPsThroughput.pdf}
%     \label{fig:simAPs}
% }
%     \caption{\rev{The communication throughput for multiple APs and UEs.}}
%     \label{fig:simthroughput}
%     \vspace{-2ex}
% \end{figure}

% \begin{figure}[h]
% \vspace{-.5ex}
% \setlength\abovecaptionskip{3pt}
% \centering
% \subfigure[One AP with different UEs.]{
%     \includegraphics[width=0.228\textwidth]{figures/simulation/simulation1APSSNR.pdf}
%     \label{fig:sim1APSSNR}
% }
% % \hspace{.1cm}
% \subfigure[50 UEs with different APs.]{
%     \includegraphics[width=0.223\textwidth]{figures/simulation/simulationAPsSSNR.pdf}
%     \label{fig:simAPsSSNR}
% }
%     \caption{{The sensing S-SNR for multiple APs and UEs.}}
%     \label{fig:simSSNR}
%     \vspace{-2ex}
% \end{figure}

\begin{figure}[t]
\setlength\abovecaptionskip{3pt}
\centering
\subfigure[Throughput.]{
    \includegraphics[width=0.228\textwidth]{figures/simulation/simulation1APThroughput.pdf}
    \label{fig:simAPthru}
}
% \hspace{.1cm}
\subfigure[S-SNR.]{
    \includegraphics[width=0.223\textwidth]{figures/simulation/simulation1APSSNR.pdf}
    \label{fig:simUEsSSNR}
}
    %\caption{The simulation performance of large-scale deployments}
    %\label{fig:simcomSSNR}
%\end{figure}

%\begin{figure}[h]
%\vspace{-.5ex}
 %\setlength\abovecaptionskip{3pt}
 %\centering
 \subfigure[Throughput.]{
     \includegraphics[width=0.228\textwidth]{figures/simulation/simulationAPsThroughput.pdf}
     \label{fig:simAPsThru}
 }
 % \hspace{.1cm}
 \subfigure[S-SNR .]{
     \includegraphics[width=0.223\textwidth]{figures/simulation/simulationAPsSSNR.pdf}
     \label{fig:simAPsSSNR}
 }
     \caption{The simulation performance of large-scale deployments: (a-b) single AP with multiple UEs, and (c-d) multiple APs with 50 UEs.}
    \label{fig:simcomSSNR}
     %\vspace{-2ex}
\end{figure}

\rev{
In this section, we use a simulation to illustrate the performance of \name for large-scale deployment. For Case~1, we increase the quantity of UEs from 1 to 50, and fix one AP as well as 10 subjects to conduct our experiment. For Case~2, we consider increasing the quantity of APs, but fix 50 UEs and 10 subjects. According to Section~\ref{sssc:model_chan}, we generate $\boldsymbol{H}_{\mathrm{s}}(t)$, $\boldsymbol{H}_{\mathrm{c}}(t)$, and $\boldsymbol{H}_{\mathrm{ms}}(t)$, since $\boldsymbol{H}_{\mathrm{ti}}(t)$ has been removed before beam scheduling. For convenience, $\boldsymbol{H}_{\mathrm{c}}(t)$ is employed Rician fading, but $\boldsymbol{H}_{\mathrm{s}}(t)$ and $\boldsymbol{H}_{\mathrm{ms}}(t)$ are used channel states trace of push-pull hand gesture collected from our previous experiments~(see Section~\ref{ssec:nfs}). For setting a specific quantity of UEs, we run the simulation over 10,000 trials, and calculate average throughputs of UEs per trial as well as S-SNRs.

The simulation results of Case~1 are shown in Figure~\ref{fig:simAPthru} and~\ref{fig:simUEsSSNR} that with increasing quantities of UEs, their throughputs decrease, but S-SNRs apparently increase. For the situation of throughputs, the reason is that larger UEs occupy more narrow beam sectors~(see Figure~\ref{fig:sector}), and \name needs to cover all of them as BC-Sets. Due to the larger number of BC-Sets, more temporal scheduling operations are run by \name. However, the larger quantity of UEs offers more sensing diversity for \name~(see Section~\ref{ssec:hybrid_sensing}), resulting in higher S-SNRs. \newrev{The results of Case~2 with increasing numbers of APs are shown in Figure~\ref{fig:simAPsThru} and~\ref{fig:simAPsSSNR} , which demonstrate that both throughput and S-SNR enhance with additional APs. More APs enable more connections to UEs and scheduling possibilities for \name, resulting in higher throughput. Meanwhile, the higher sensing diversity introduced by an increasing number of APs also improves S-SNRs. }
}

% Following the IEEE 802.11ay DMG specifications~\cite{802_11ay}, we evaluated the performance of \name in complex scenarios with multiple UEs served by separate Tx chains in Matlab simulation. The configuration employs a hybrid beamforming setup and extracts the channel state information (CSI) at the AP to compute the SNR.
%

% For simplicity,  both APs and UEs use stochastic Rician channel. Each UE finds the APs with the optimal SNR through the beamforming procedure described in Sec~\ref{append:A}. 

% Figure~\ref{fig:simthroughput} shows the simulation results of throughput (Gbps) on a large scale (multiple APs, multiple UEs).
%
% With the increasing number of UEs, there is a moderate decline in throughput observed, which remains within an acceptable range.

%
% The simulation of the sensing performance is partially based on the Matlab example for Joint Radar-Communication (JCS) as presented in~\cite{JRC_Matlab}. 
% %
% In our Matlab-based simulation, OFDM waveforms were utilized for simplicity, and the reflection coefficient was adjusted to emulate the conditions pertinent to subject sensing.
% %
% For each pair of APs and UEs, the simulation models the transmission of the OFDM signal and its subsequent reception at the Rx. The S-SNR~\cite{RFSINR-SenSys22} is subsequently computed based on the power of the reflection.
% %
% The results, depicting the S-SNR (dB) for multiple UEs, can be viewed in Figure~\ref{fig:simSSNR}. 
